# Supplementary material for: Fast and flexible long-range models for atomistic machine learning
Source: arXiv:2412.03281 source file (2025-03-24)
Supplement: Supplementary file 2 [file implementation.tex]

\section{Implementation Details}
